# Supplementary material for: The 8-Point Algorithm as an Inductive Bias for Relative Pose Prediction by ViTs
Source: arXiv:2208.08988 source file (2023-01-24)
Supplement: Supplementary file 1 [file supp_arch2.tex]

\parnobf{Backbone}

\parnobf{Essential Matrix Module}

\parnobf{Baselines}

\parnoit{CNN Pose Regressor}

\parnoit{+ViT}

\parnoit{+Bilinear Attention}

\parnoit{+Dual Softmax}

\begin{table}[t]
\caption{\textbf{Model Architecture}. }\label{tab:model_arch}
\centering
\scriptsize

\begin{tabular}{lc}
\toprule
\multicolumn{2}{c}{Overview} \\
 Operation & Output Shape           \\ \midrule
 Input Image & $ 2 \times 3 \times 256 \times 256$ \\
 Encoder & $ 2 \times H \times H \times D $           \\
 ViT Layer (x5) & $2 \times H \times H \times D$           \\
 Essential Matrix Module & $2 \times N_h \times (D/N_h + 6) \times (D/N_h + 6)$           \\
MLP & $7$           \\
\bottomrule
~ \\
\toprule
\multicolumn{2}{c}{Encoder} \\
 Operation & Output Shape           \\ \midrule
 ResNet-18 Block 1 & $ 2 \times 56 \times 56 \times 64$ \\
 ResNet-18 Block 2 & $ 2 \times H \times 28 \times 128$ \\
 Residual Module & $ 2 \times H \times H \times D$ \\
\bottomrule
~ \\
\toprule
\multicolumn{2}{c}{MLP} \\
 Operation & Output Shape           \\ \midrule
 Linear \& ReLU (x2) & 512 \\
 Linear \& ReLU & 7 \\
\bottomrule
~ \\
\toprule
\multicolumn{2}{c}{Residual Module} \\
 Operation & Output Shape           \\ \midrule
\textit{Branch A} \\
 2D Conv k=3 s=1, BN, ReLU & $ 2 \times 28 \times 28 \times D$ \\
 2D Conv k=5 s=1, BN, ReLU & $ 2 \times H \times H \times D$ \\
 \\
\textit{Branch B} \\
 2D Conv k=5 s=1, BN & $ 2 \times H \times H \times D$ \\
 \\
\textit{Forward Pass} \\
ReLU(Branch A + Branch B) & $2 \times H \times H \times D$ \\
\bottomrule
\end{tabular}
\end{table}

\begin{table*}[t]
\vspace{2mm}
\begin{tabular}{lc}
\toprule
\multicolumn{2}{c}{ViT Layer} \\
 Operation & Output Shape           \\ \midrule
{\it Attn} \\
Q,K,V $=$ Linear & $ 2 \times N_h \times (H \times H) \times (D/N_h)$ \\
A $= \textrm{SM}(Q @ K^T, dim=-1)$ & $ 2 \times N_h \times (H \times H) \times (H \times H)$ \\
$(A @ V)^T$ & $ 2 \times H \times H \times D$ \\
Linear & $ 2 \times H \times H \times D$ \\
\\
\textit{MLP} \\
Linear \& GeLU & $ 2 \times H \times H \times (D \times 4)$ \\
Linear & $ 2 \times H \times H \times D$ \\
\\
\textit{Forward Pass} \\
 Attn(LayerNorm) + Residual & $ 2 \times H \times H \times D$ \\
 MLP(LayerNorm) + Residual & $ 2 \times H \times H \times D$ \\
\bottomrule
~ \\
\toprule
\multicolumn{2}{c}{Essential Matrix Module} \\
 Operation & Output Shape           \\ \midrule
\textit{MLP} \\
Linear \& GeLU & $ 2 \times H \times H \times (D \times 4)$ \\
Linear & $ 2 \times H \times H \times D$ \\
\\
\textit{Forward Pass} \\
 Essential Matrix Cross-Attn(LayerNorm) + Residual & $2 \times N_h \times (D/N_h + 6) \times (D/N_h + 6)$ \\
 MLP(LayerNorm) + Residual & $2 \times N_h \times (D/N_h + 6) \times (D/N_h + 6)$ \\
\bottomrule
~ \\
\toprule
\multicolumn{2}{c}{Essential Matrix Cross-Attn} \\
 Operation & Output Shape           \\ \midrule
\textit{Attn Branch} \\
A $= \textrm{SM}(Q @ K^T, dim=-1) \times \textrm{SM}(Q @ K^T, dim=-2) $ & $ N_h \times (H \times H) \times (H \times H)$ \\
$(V^T @ A @ V)^T$ & $N_h \times (D/N_h + 6) \times (D/N_h + 6)$ \\
Linear & $N_h \times (D/N_h + 6) \times (D/N_h + 6)$ \\
\\
\textit{Forward Pass} \\
$Q_1,K_1,V_1 = Linear(Input[0])$ & $ N_h \times (H \times H) \times (D/N_h + 6)$ \\
$Q_2,K_2,V_2 = Linear(Input[1])$ & $ N_h \times (H \times H) \times (D/N_h + 6)$ \\
$V1[...,-6:], V2[...,-6:] = Pos Encoding$ & $ N_h \times (H \times H) \times (D/N_h + 6)$ \\
$Concat(Attn Branch(Q_1, K_2, V_2), Attn Branch(Q_2, K_1, V_1))$ & $2 \times N_h \times (D/N_h + 6) \times (D/N_h + 6)$ \\
\bottomrule
\end{tabular}
\end{table*}
